# Supplementary material for: Deep Bregman Divergence for Contrastive Learning of Visual Representations
Source: arXiv:2109.07455 source file (2021-11-22)
Supplement: Supplementary file 1 [file appendix.tex]

\section{APPENDIX}~\label{appendix}

\noindent\textbf{Impact of Bregman divergence network on quality of representations} We visualize the representation features using t-SNE with the last convolution layer from ResNet-18 to explore the quality of learned features using our proposed method. Figure~\ref{fig:tsne} compares the representation space learned by our proposed method (a) and SimCLR (b). As depicted in Fig.~\ref{fig:tsne}, our model shows better separation on clusters, especially for classes 2, 4, 6, and 7.

\begin{figure}
  \centering
  \subfloat[]{\includegraphics[width=0.45\textwidth]{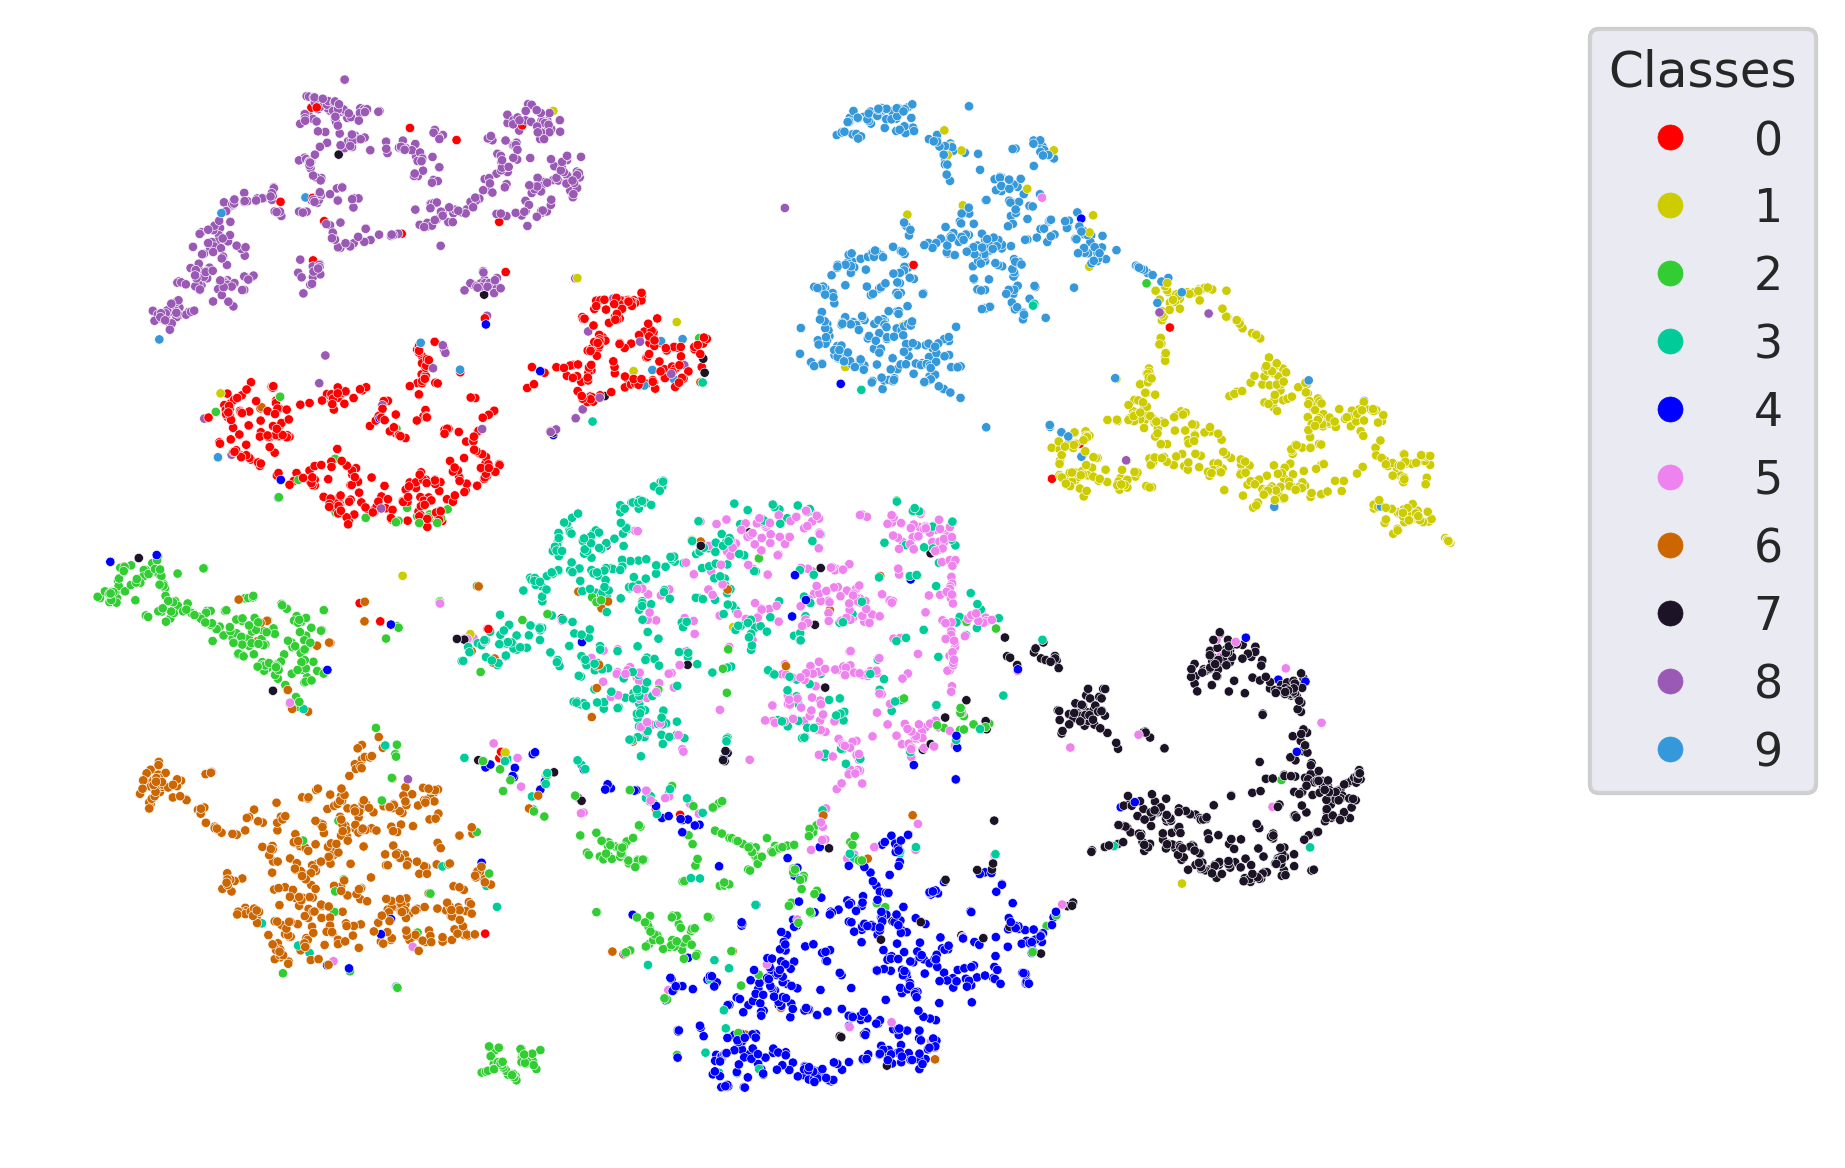}\label{fig_1a}}
  \hfill
  \subfloat[]{\includegraphics[width=0.45\textwidth]{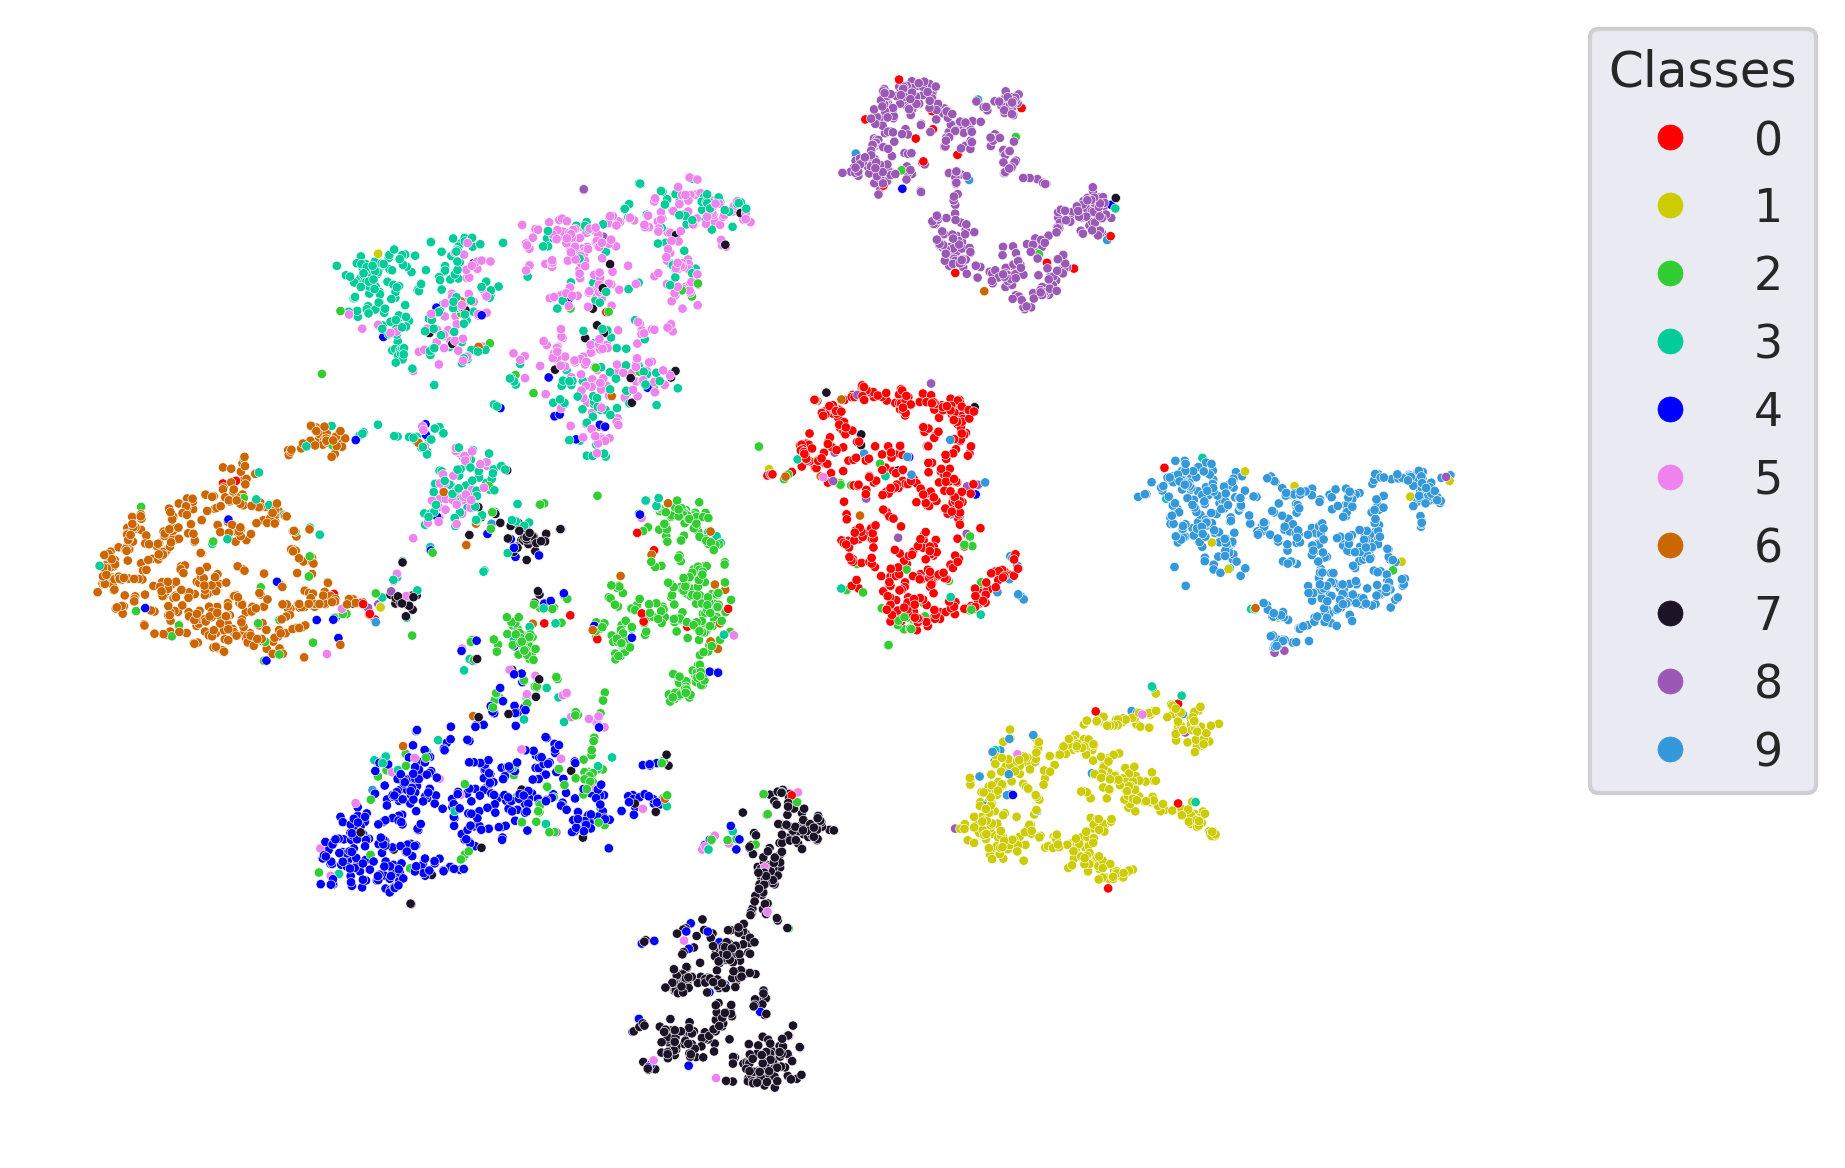}\label{fig_2b}}
  \caption{t-SNE visualization of embeddings with ResNet-50 on CIFAR-10: (a) SimCLR, (b) our method. Classes are well-clustered using our method especially for classes 2, 3, and 5. }
\label{fig:tsne}
\end{figure}

%\noindent\textbf{Training Details}
%We use Adam optimizer~\cite{kingma2014adam} with a learning rate $0.005$, and weight decay $0.0001$ without restarts, over 300 epochs for all of the pretraining. Figure~\ref{fig:loss} shows a sample learning curve of our model using the ResNet-18 base network over 100 epochs and the corresponding test loss and top-1 and top-5 accuracy on CIFAR-10 dataset. For the pre-training we use with a mini-batch size of 512 and 2 GPUs. 

%\begin{figure}
%  \centering
%  \includegraphics[width=0.49\textwidth]{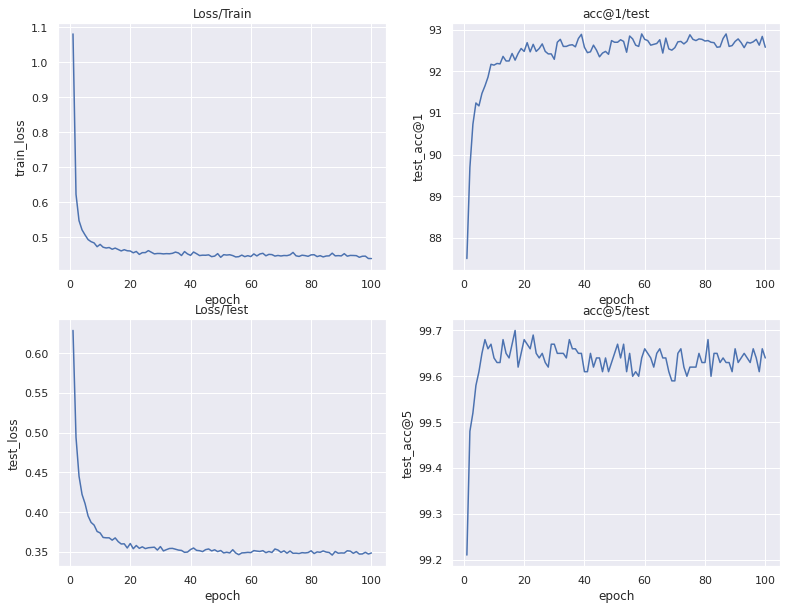}
%  \caption{The learning curves of deep Bregman divergence and the corresponding test loss, top-1 and top-5 accuracy for linear evaluation on CIFAR-10.}
%\label{fig:loss}
%\end{figure}

\noindent\textbf{Other Applications}
The metric learning and divergence learning problems are the fundamental problem in machine learning, attracting considerable research and applications. These applications include (but not limited to) uncertainty quantification, density estimation, image retrieval, unsupervised image clustering, program debugging, image generation, music analysis, and ranking. Fundamental studies in these problems will help to improve results in these applications as well as direct to additional impact in new domains.

% \begin{figure} [!t]
% \centering
% \includegraphics[width=0.49\textwidth]{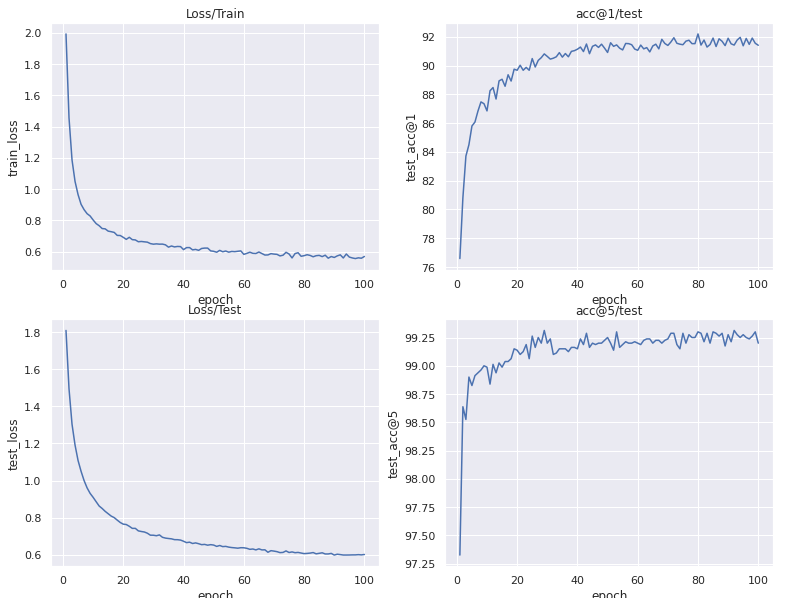}
% \caption{The curves of training and testing of loss and accuracy for linear evaluation on STL-10~(\ref{fig_stl}) } 
% \label{fig_stl}
% \end{figure}

% \begin{figure*}[!t]
%   \centering
%   \subfloat[]{\includegraphics[width=0.49\textwidth]{figures/cifar10_linear.png}\label{fig_cifar}}
% %   \hfill
%   \subfloat[]{\includegraphics[width=0.49\textwidth]{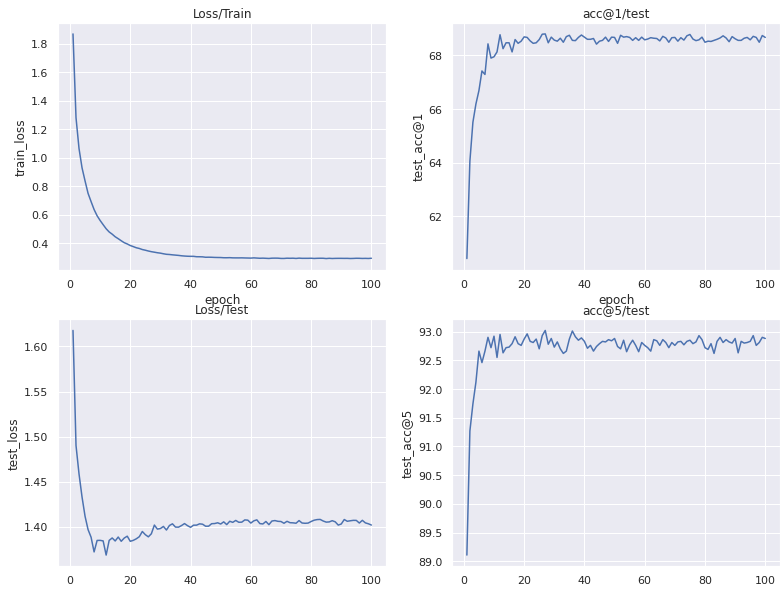}\label{fig_cifar100}}
%   \caption{The curves of training and testing of loss and accuracy for linear evaluation on CIFAR-10~(\ref{fig_cifar}) and CIFAR-100~(\ref{fig_cifar100})}
% \label{fig:loss}
% \end{figure*}

% \newpage
\newpage

%\begin{algorithm} 
 %   \SetKwInOut{Input}{Input}
 %   \SetKwInOut{Output}{Output}

%    \Input{ $\mathcal{X}= \{ v_{x_1}, v_{x_1}, ..., v_{x_n} \} \in \mathbb{R}^{m},$ $\kappa$ } 
%    \Output { $\mathcal{X}= \{ v_{x_1}, v_{x_1}, ..., v_{x_n} \} \in \mathbb{R}^{m}, \kappa $$ } 

%  \For{sample mini-batch $\{x_i\}_{i=1}^N$} 
%    {
%    \For{all $i \in {1,..., N}$}
%    {
%    perform data augmentation using transformation function $\tau$ \\
%    learn representation using $f_{\theta}$ \\
%    learn divergence using $D_{phi}$\\
%    }
%    \For{all $i \in {1,..., N}$}
%    {
%     learn Bregman distance\\
%     create a pairwise similarity matrix\\
%    }
%    \For{all $i \in {1,..., N}$}
%    {
%    update network f,g, D, to minimize the\\
%    $ L_{ConDiv} = \ell_{Con} + \ell_{Div}$
%    }
%    \return representation network $\f(\cdot)$
%    }
%\caption{Pseudocode for our proposed Bregman divergences network}
%\label{alg}
%\end{algorithm}

% $= 1/exp(-D/{2{\sigma}^2})$ (where $\sigma$ is adjustable parameter). In our experiments, we incorporate contrastive loss into deep Bregman learning $\ell^{div(p, q)}$ (Eq.~\ref{eq:pair_div_loss}) addition to $ \ell^{\mathrm{NT}\text{-}\mathrm{Xent}}$ (Eq.~\ref{eq:NTXent}).
